# Supplementary material for: MambaMOT: State-Space Model as Motion Predictor for Multi-Object Tracking
Source: arXiv:2403.10826 source file (2025-01-21)
Supplement: Supplementary file 1 [file 7_supp.tex]

The appendix is structured as follows:

\begin{itemize}
    \item A. Model Size
    \item B. More Comparison with ByteTrack
    \item C. Intuition behind MambaTrack\textsuperscript{+}
\end{itemize}

\section{Model Size}
We experimented with different numbers of Mamba blocks as our motion model on the DanceTrack validation set \cite{sun2022dancetrack}. It was found that a motion model comprising four blocks yielded the highest performance in HOTA, while stacking more blocks for motion prediction did not bring any further performance improvement. This lack of improvement could be attributed to overfitting to the training data. Due to the marginal performance gains over computational efficiency, we chose to implement the MambaTrack motion model with only two Mamba blocks.

\begin{table*}
\caption{HOTA performance comparison on DanceTrack validation set with different number of mamba blocks.}
\vspace{-6pt}
  \begin{center}
    {
\begin{tabular}{ccccc}
\toprule 

\hspace{.5em}$\#blocks$ & 
\hspace{1em} 2 \hspace{1em} &
\hspace{1em} 4 \hspace{1em} &
\hspace{1em} 6 \hspace{1em} &
\hspace{1em} 8 \hspace{1em} \\
\midrule

HOTA & 52.0 & \textbf{52.1} & 50.9 & 50.9  \\

\bottomrule
\end{tabular}
}
\vspace{-18pt}
\label{table:cost}
\end{center}

\label{table:model size}

\end{table*} 

\newpage
\section{More Comparison with ByteTrack}
Our proposed MambaTrack employs a similar association method to the state-of-the-art method ByteTrack \cite{zhang2022bytetrack}. However, our method outperforms ByteTrack by a large margin on several challenging datasets with targets exhibiting nonlinear movements. Under the same online tracking setting, MambaTrack achieves an 8.2\% HOTA improvement over ByteTrack on the DanceTrack dataset and an 8.4\% HOTA improvement on the SportsMOT dataset \cite{cui2023sportsmot} using the same detection generated by YOLOX \cite{ge2021yolox}. We provide more visualization results comparing MambaTrack and ByteTrack in Fig. \ref{fig:example} and Fig. \ref{fig:trajectory}.

\vspace{-12pt}

\begin{figure}
\centering
\includegraphics[width=\linewidth]{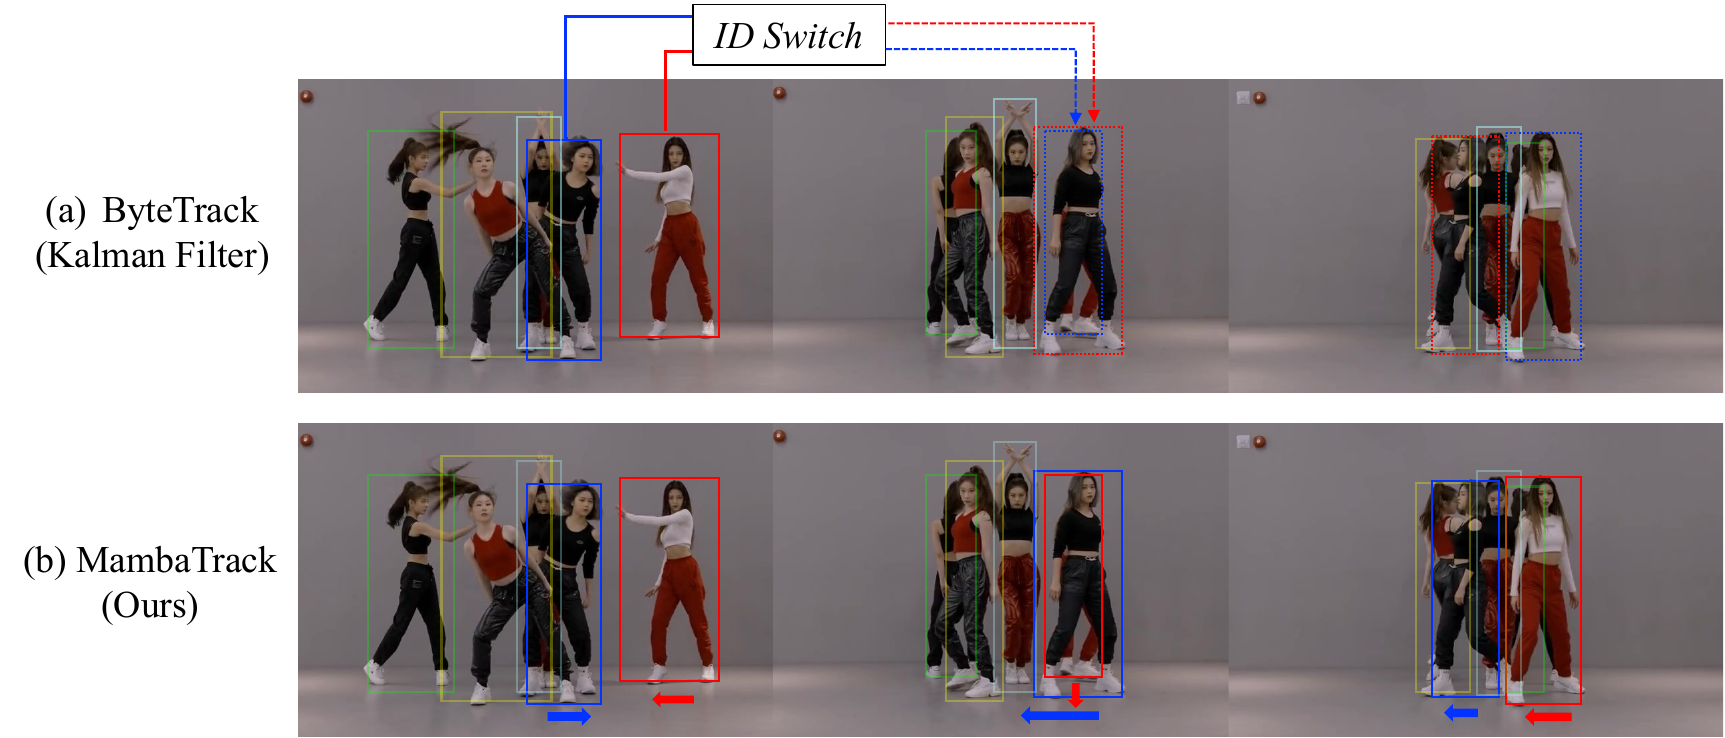}
\caption{We demonstrate the challenge in DanceTrack where Kalman-based Motion Predictor can fail due to large movement in DanceTrack dataset due to occlusion and non-linear motion. The visualized results are (a) ByteTrack and (b) our proposed MambaTrack on the \textit{dancetrack0038} sequence from the testing split. The colored arrows represent the track motion direction. On the second frame, ByteTrack encounters an ID switch for the target with red pants, while MambaTrack does not.}
\label{fig:example}
\end{figure}

\vspace{-24pt}

\section{Intuition behind MambaTrack\textsuperscript{+}}

Tracklet merging is a technique used to further boost tracking performance by merging fragment tracklets of the same identity and assigning them the same tracking ID. This technique \cite{du2023strongsort,zhang2023translink,suljagic2022similarity,you2024multi,zhang2023multi,huang2023observation,yang2024sea}  has shown effectiveness in boosting association performance metrics like IDF1 and AssA. Tracklet merging usually utilize object appearance features or motion features for tracklet association and serve as a post-processing approach after tracking is completed by an online tracker. 

Although these plug-and-play tracklet merging methods can be applied to various online trackers and improve their performance, they still require an additional training procedure and entail extra computational costs beyond the original tracking process. In contrast, our proposed MambaTrack\textsuperscript{+}, unifies online tracking and offline tracklet merging frameworks by reusing tracklet features, making it more computationally efficient compared to existing methods. Some sampled cases of MambaTrack\textsuperscript{+} are provided in Fig. \ref{fig:plus}.

\begin{figure}
\centering
\includegraphics[width=\linewidth]{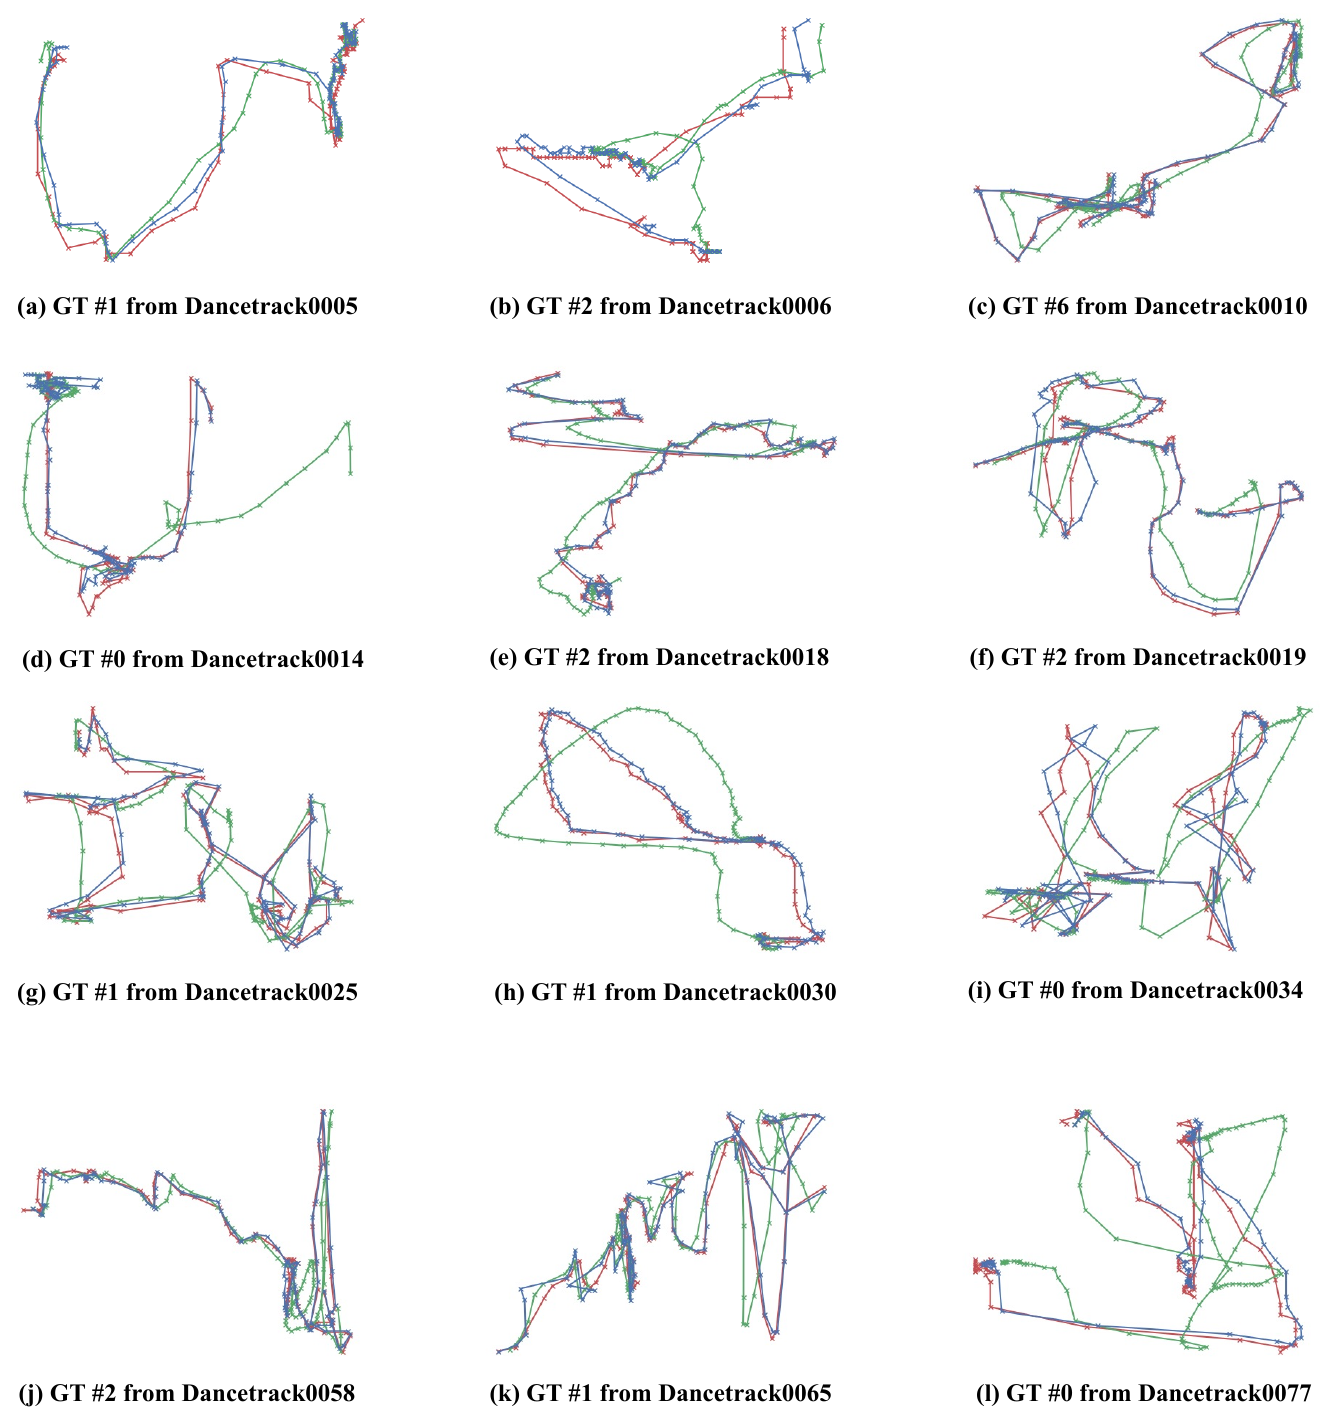}
\caption{Trajectory visualizations of the first 100 frames sampled from the DanceTrack validation set. We showcase a more detailed comparison between the tracking results of ByteTrack (Kalman filter-based) and our proposed MambaTrack. With the \textcolor{OliveGreen}{green dots} representing the object trajectory from ByteTrack's prediction and the \textcolor{blue}{blue dots} depicting the object trajectory from MambaTrack's prediction. The \textcolor{red}{red dots} denote the ground truth trajectory.}
\label{fig:trajectory}
\end{figure}

\begin{figure}
\centering
\includegraphics[width=\linewidth]{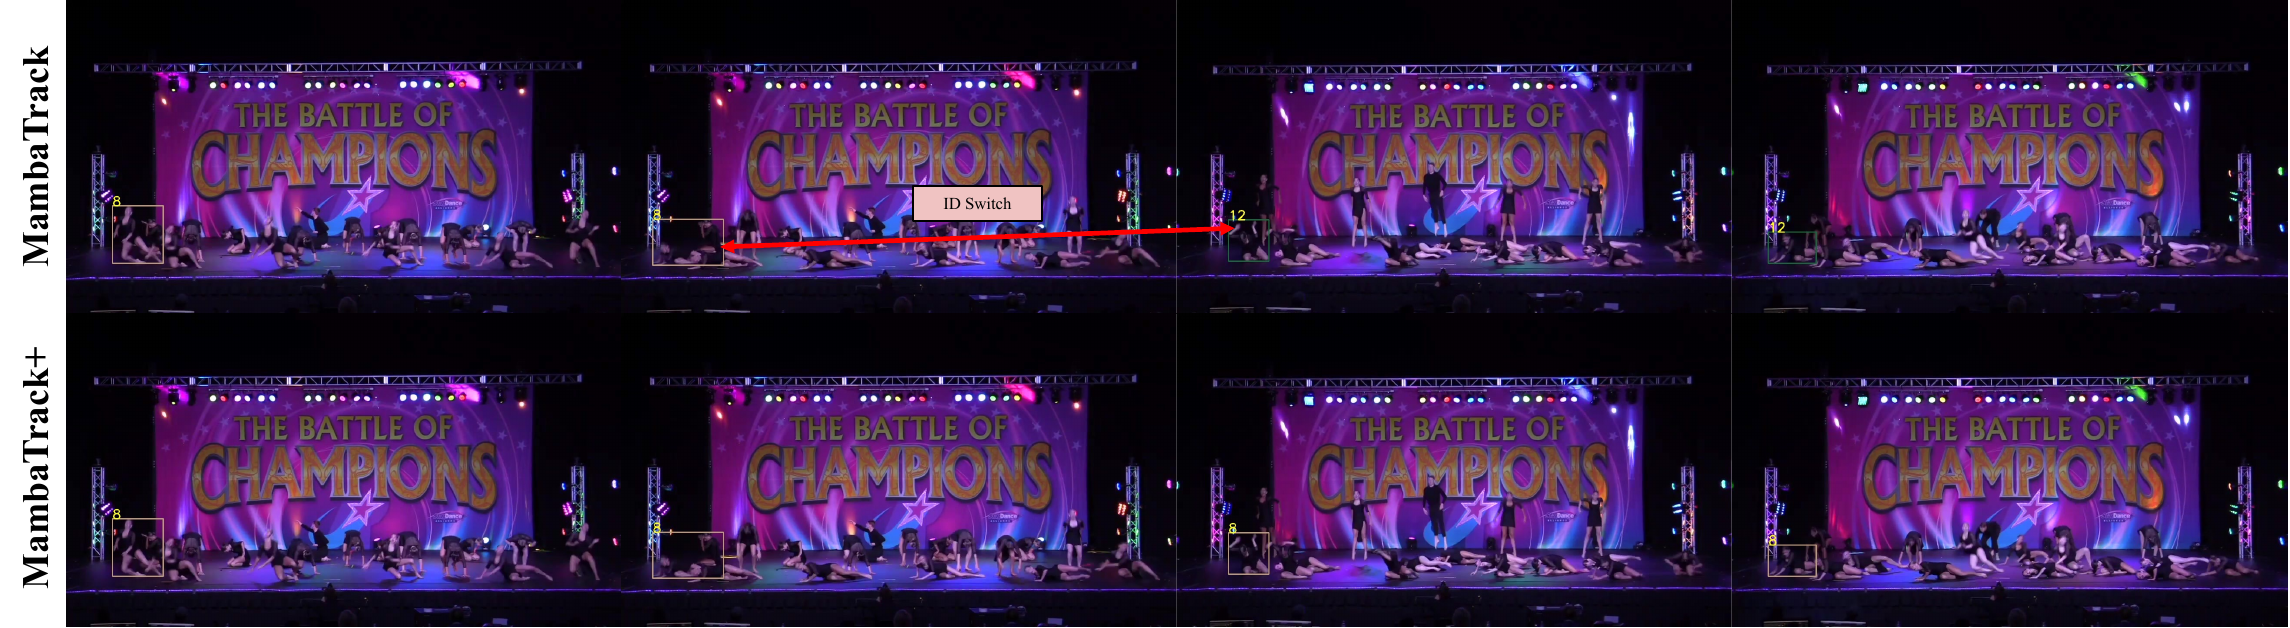}
\includegraphics[width=\linewidth]{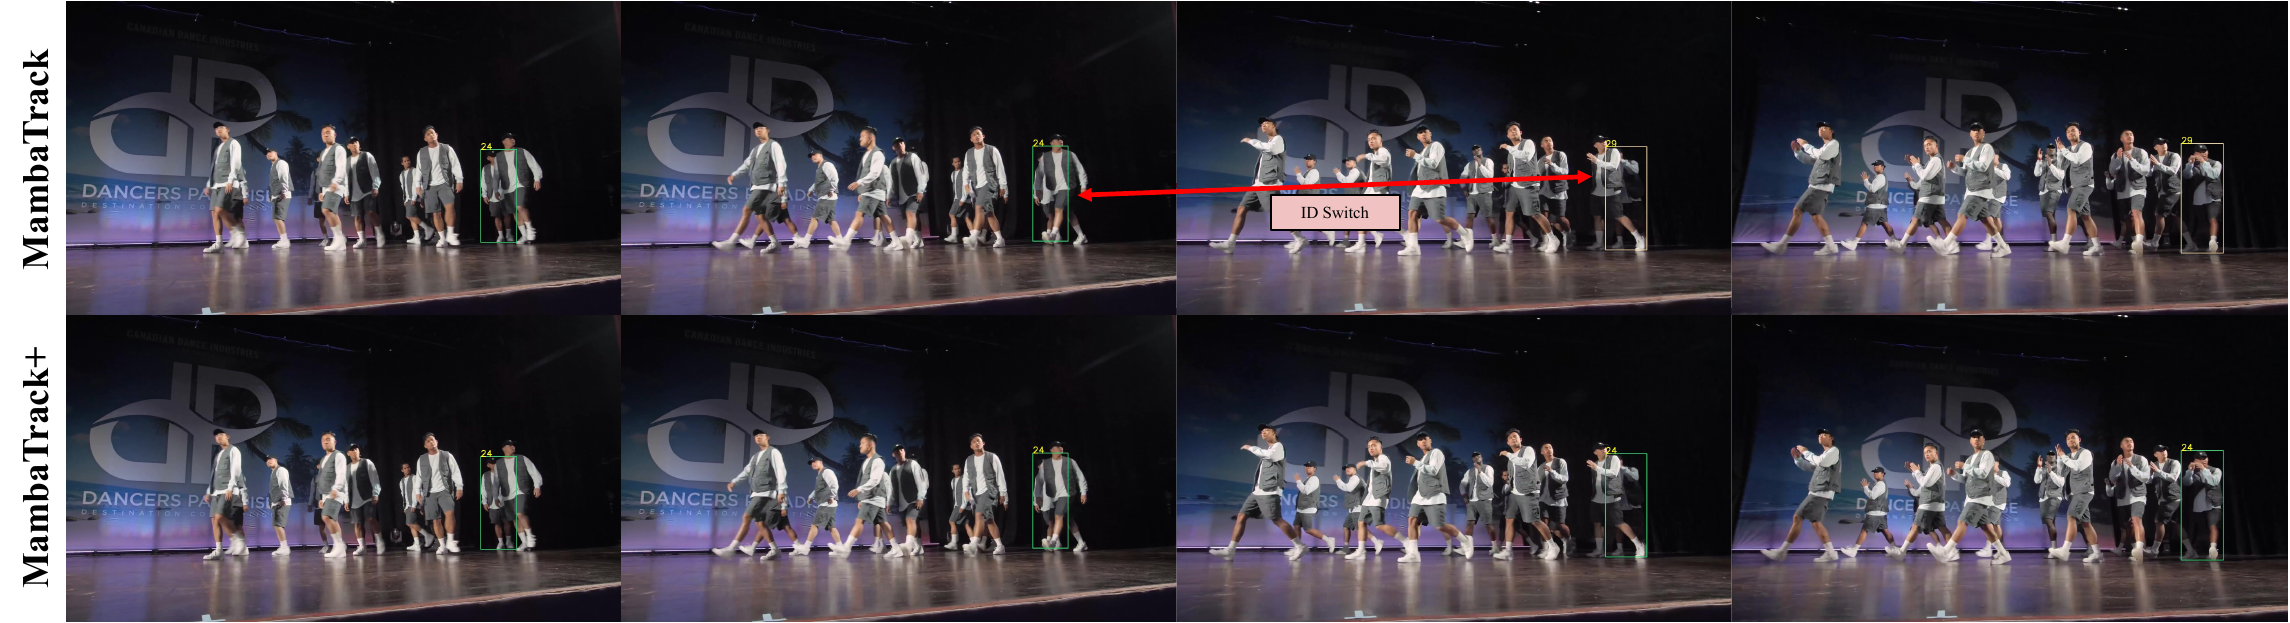}
\includegraphics[width=\linewidth]{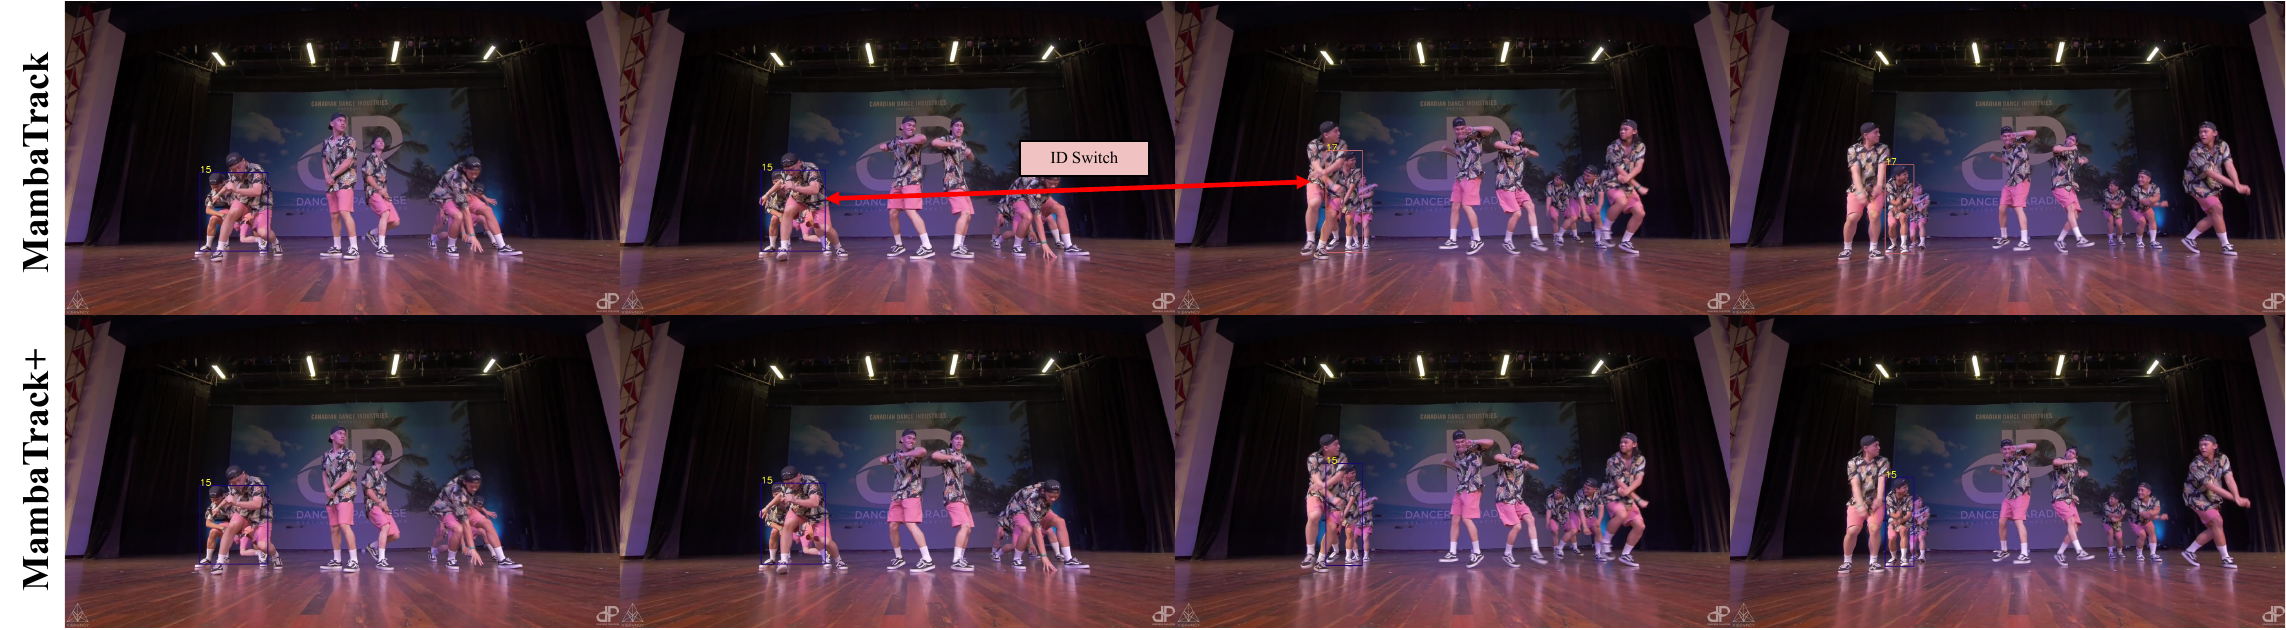}
\includegraphics[width=\linewidth]{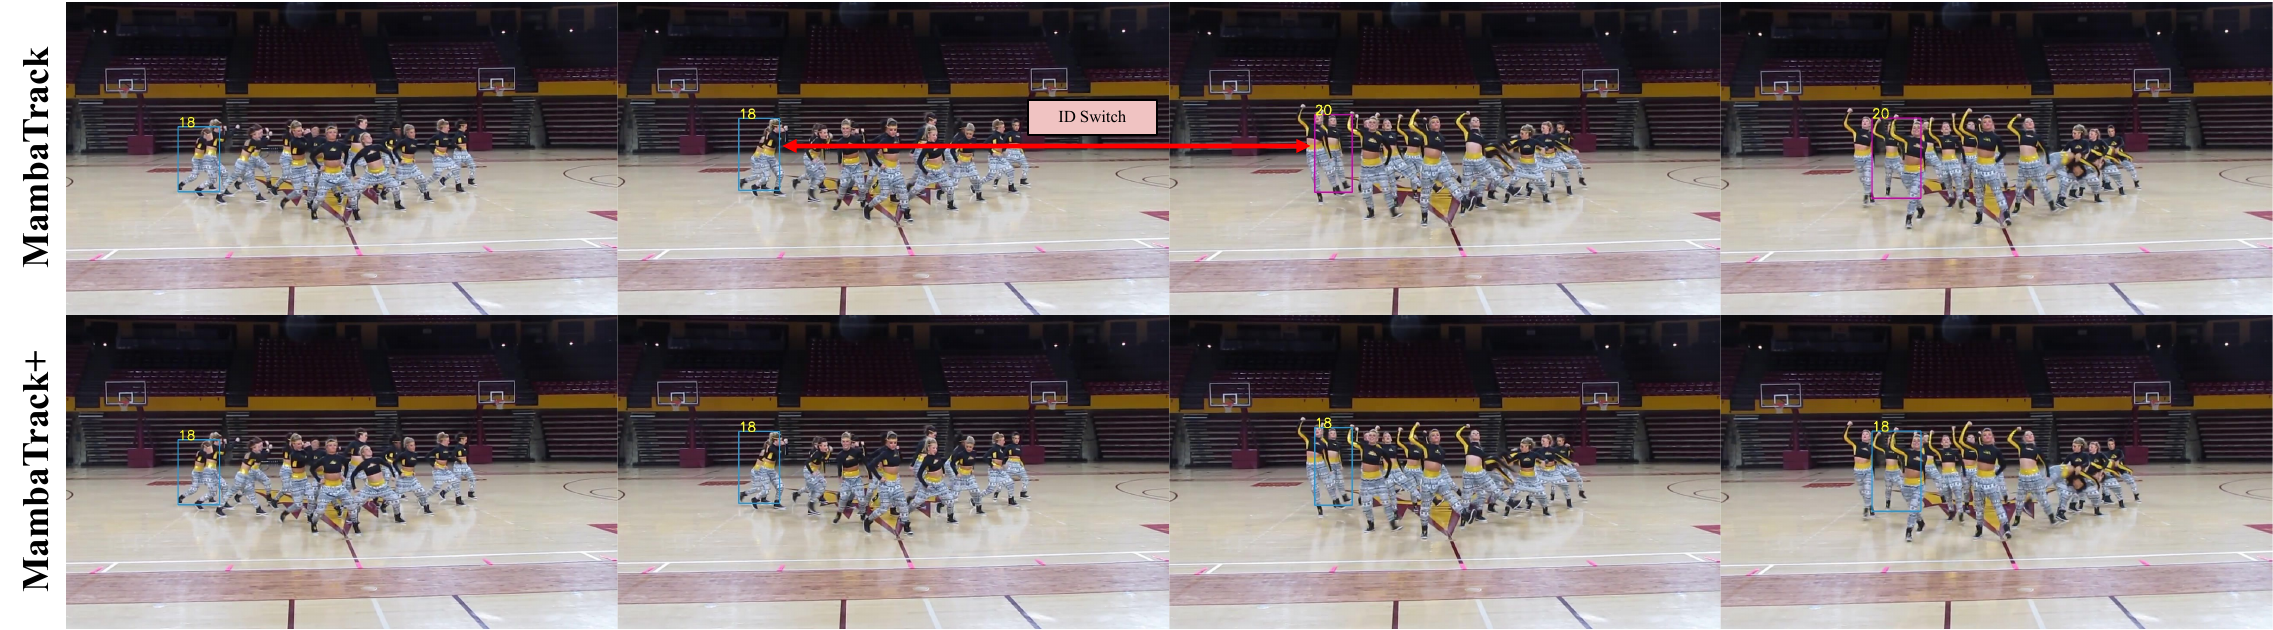}
\caption{Some tracking results from MambaTrack (upper row) and MambaTrack\textsuperscript{+} (lower row) sampled from the DanceTrack validation set. MambaTrack\textsuperscript{+} successfully merges fragment tracklets when ID switches are caused by occlusion, irregular movements, or inaccurate detections during the tracking process.}
\label{fig:plus}
\end{figure}
